# Supplementary material for: Interpretable multiscale Machine Learning-Based Parameterizations of Convection for ICON
Source: arXiv:2311.03251 ancillary file (2024-09-20)
Supplement: Supplementary file 1 [file supplementary_information.pdf]

# Supporting Information for "Interpretable multiscale Machine Learning-Based Parameterizations of Convection for ICON"

**Helge Heuer**[1], **Mierk Schwabe**[1], **Pierre Gentine**[2], **Marco A. Giorgetta**[3], **Veronika Eyring**[1,4]

[1]Deutsches Zentrum für Luft- und Raumfahrt e.V. (DLR), Institut für Physik der Atmosphäre, Oberpfaffenhofen, Germany

[2]Center for Learning the Earth with Artificial Intelligence and Physics (LEAP), Columbia University, New York, NY, USA

[3]Max Planck Institute for Meteorology, Hamburg, Germany

[4]University of Bremen, Institute of Environmental Physics (IUP), Bremen, Germany

## Contents of this file

1. Sections 1 to 2
2. Figures 1 to 7
3. Tables 1 to 2

## Introduction

In the first section S1, this file contains supplementary Figures 1, 2, 3, 4, 6, and 7, as well as a short description of those to compare with figures in the main part and give additional information. Section S2 provides a brief summary on the used non-deep learning models. Section S3 gives some additional information on the used machine learning models and their hyperparameters. Figure 8 visualizes the model training/validation/testing procedure. Tables 1 and 2 are included in this section to give more information on the number of trainable parameters and used hyperparameters.

## Section S1

Some additional figures, presenting more details to the results shown in the main document, are presented in this section.

Figure 1 displays the predicted subgrid fluxes against the true subgrid fluxes. The fluxes for the tracer species $q_l$, $q_i$, $q_r$, $q_s$ are shown. The tendency to underestimate the true flux for high values which was previously observed is also visible in this figure.

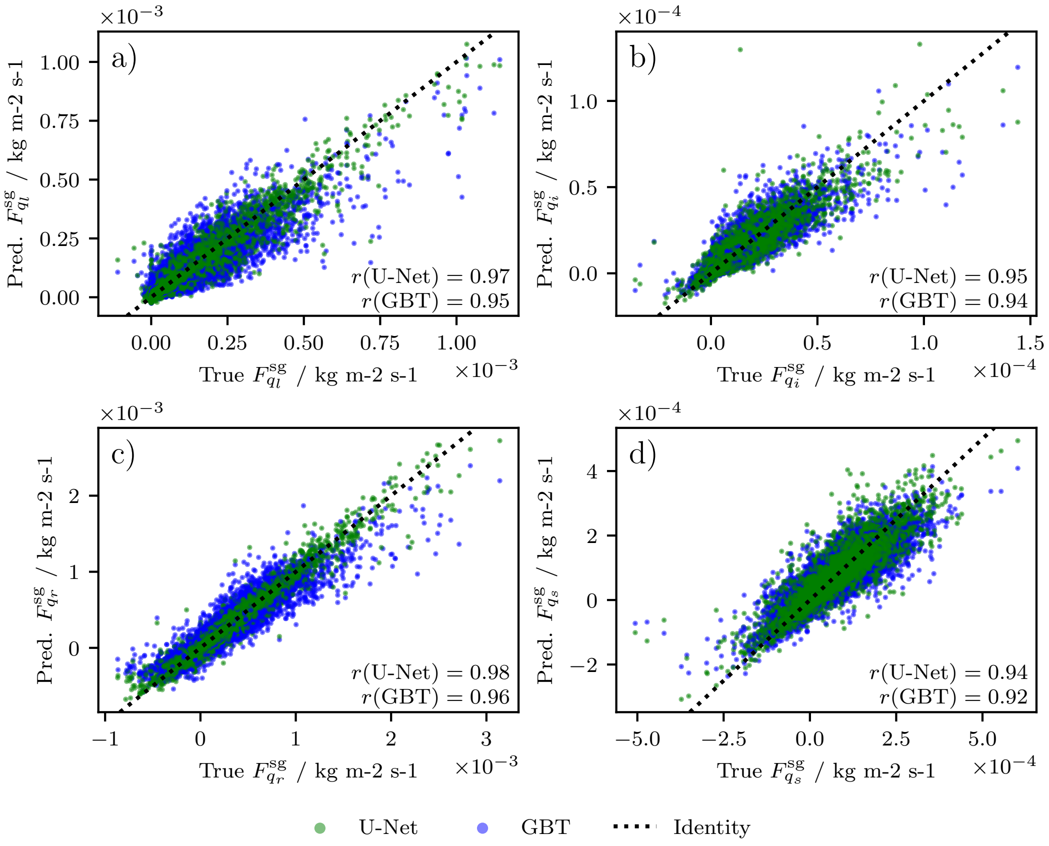


**Figure 1.** Scatterplots for the subgrid fluxes of the four remaining tracer species not shown in the main document. Data for the U-Net is shown in green, for the GBT in blue, and the diagonal is marked by a dotted line. The Pearson correlation coefficient is written in the lower right of each plot for both U-Net and GBT.

The true and predicted precipitation distributions are displayed in Figure 2. Although the difference in the $R^2$ value is just $\sim 0.04$ we see that the tail of the true distribution is much better captured by the U-Net in comparison to the GBT model.

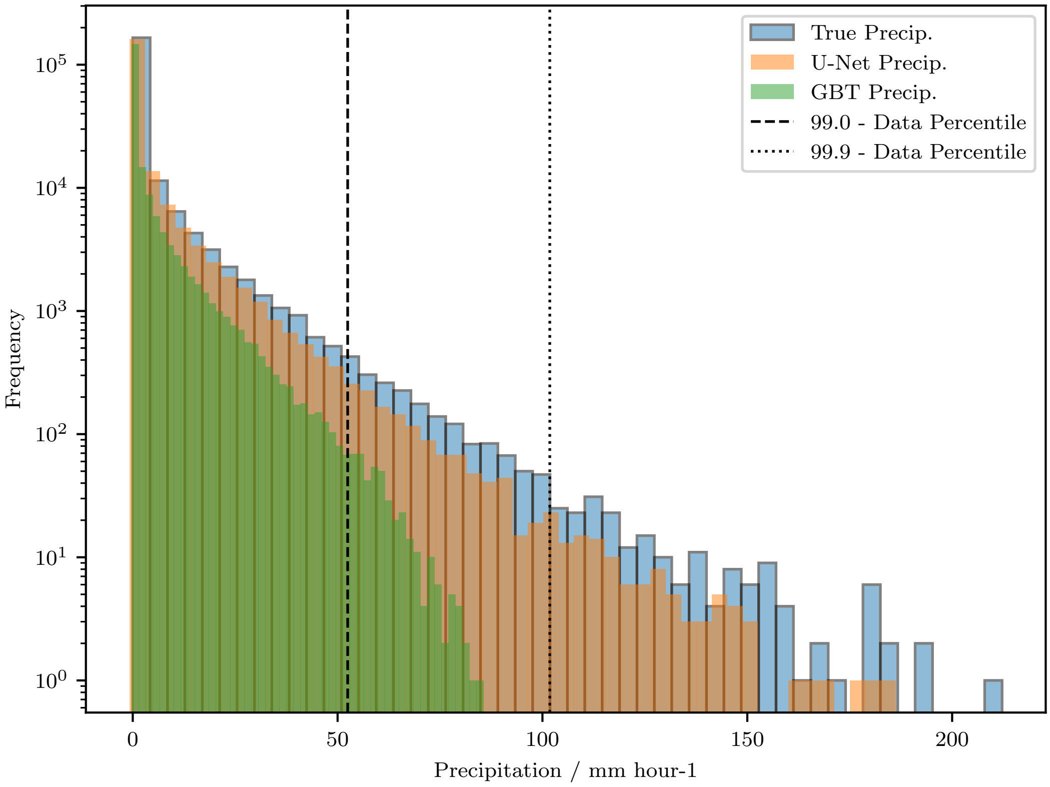


**Figure 2.** Distribution of the true precipitation and the predictions of U-Net and GBT. The 99th and the 99.9th percentile of the true precipitation are marked by the dashed and the dotted line, respectively. The precipitation $R^2$ scores are 0.897 for the U-Net and 0.860 for the GBT.

The variance weighted RMSE of U-Net and GBT is shown in Figure 3. We computed the RMSE across all variables and levels in this plot, excluded columns are shown as grey data points.

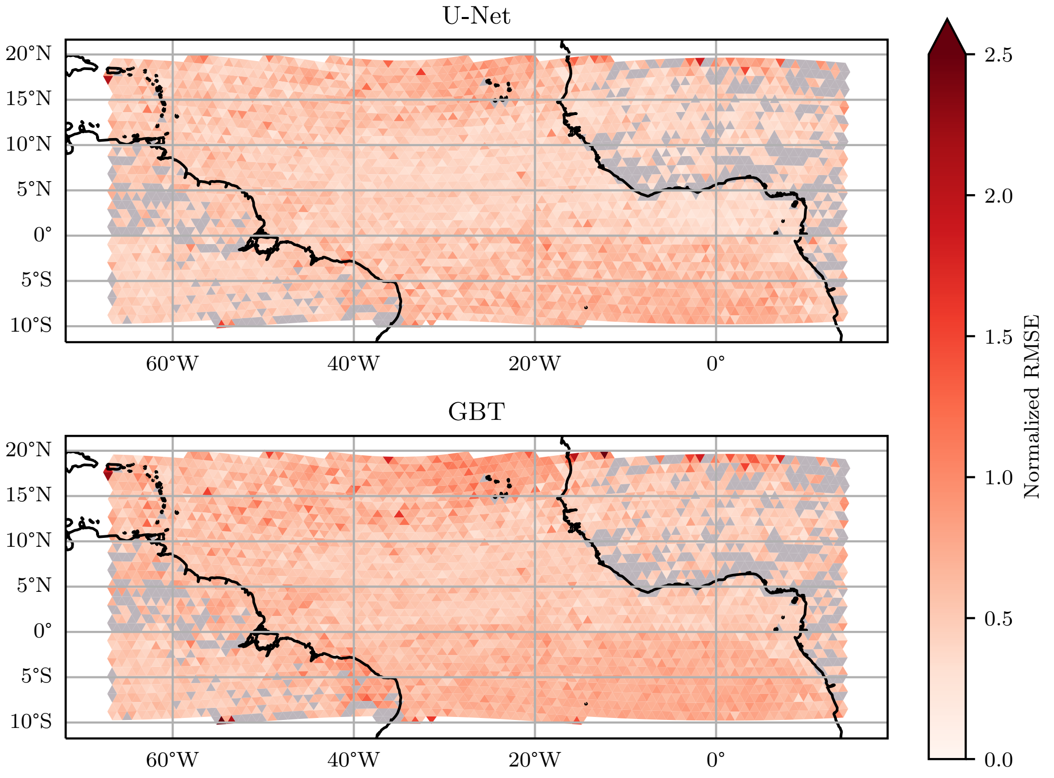


**Figure 3.** Spatial distribution of the by the variance weighted RMSE in the studied region. The top plot shows the data for the U-Net and on the bottom the result of the GBT model is displayed.

Figure 4 displays the weighted SHAP values and the feature importance for the non-ablated U-Net. By looking at the column for $q_r/q_s$ we see that the model is heavily influenced by these variables and other variables have a comparatively lower influence on the target fluxes.

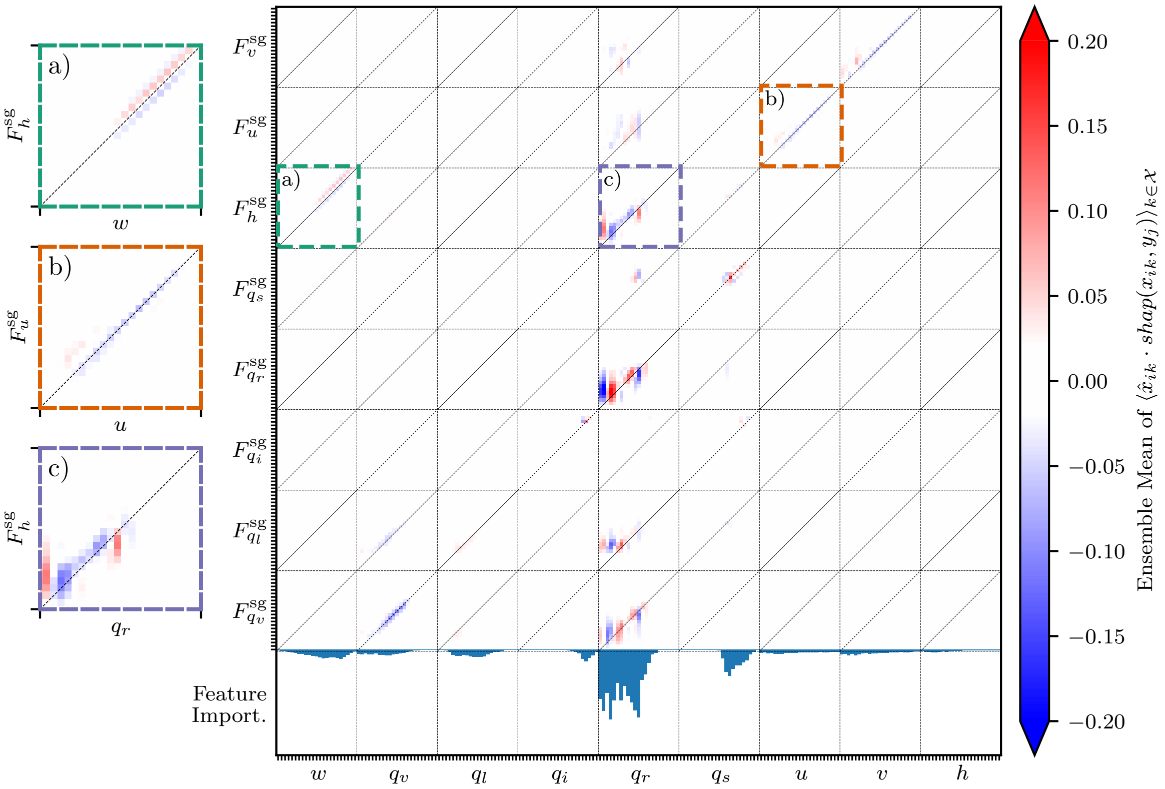


**Figure 4.** Ensemble mean of weighted SHAP values for the non-ablated U-Net model. The feature importance shown in the lower part of the figure shows the mean absolute SHAP values averaged over all target fluxes. The Insets a), b), and c) show a more detailed version of three specific variable pairs, the colors indicate which inset corresponds to which part of the large plot.

Figure 5 displays the weighted SHAP values and the feature importance for the non-ablated MLP. By looking at the column for $q_r/q_s$ we see that the model is heavily influenced by these variables, as well, and other variables have a comparatively lower influence on the target fluxes.

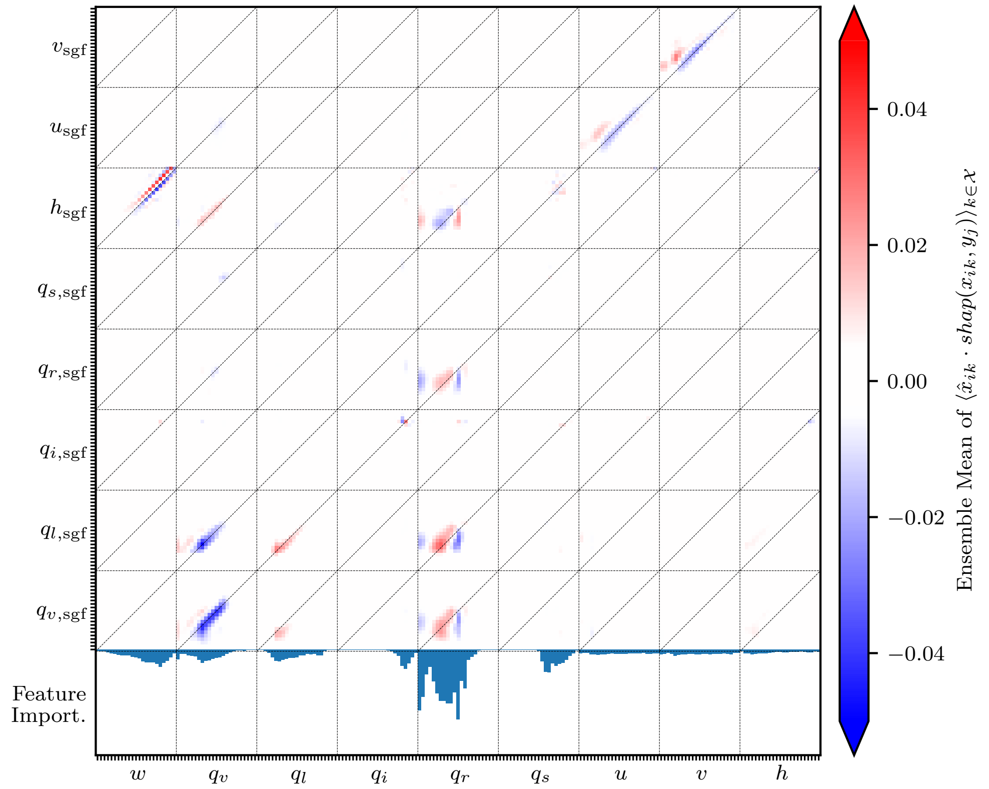


**Figure 5.** Ensemble mean of weighted SHAP values for the non-ablated MLP model. The feature importance shown in the lower part of the figure shows the mean absolute SHAP values averaged over all target fluxes. The Insets a), b), and c) show a more detailed version of three specific variable pairs, the colors indicate which inset corresponds to which part of the large plot.

Figure 6 shows a complexity-performance plot of the used non-tree-based models. Tree-based models are not compared in this plot as the number of parameters is not a meaningful measure of complexity for this model class. A Pareto frontier, defined as the set of points for which no other point exists with one improved metric and no metric worsened, is displayed in the figure, as well.

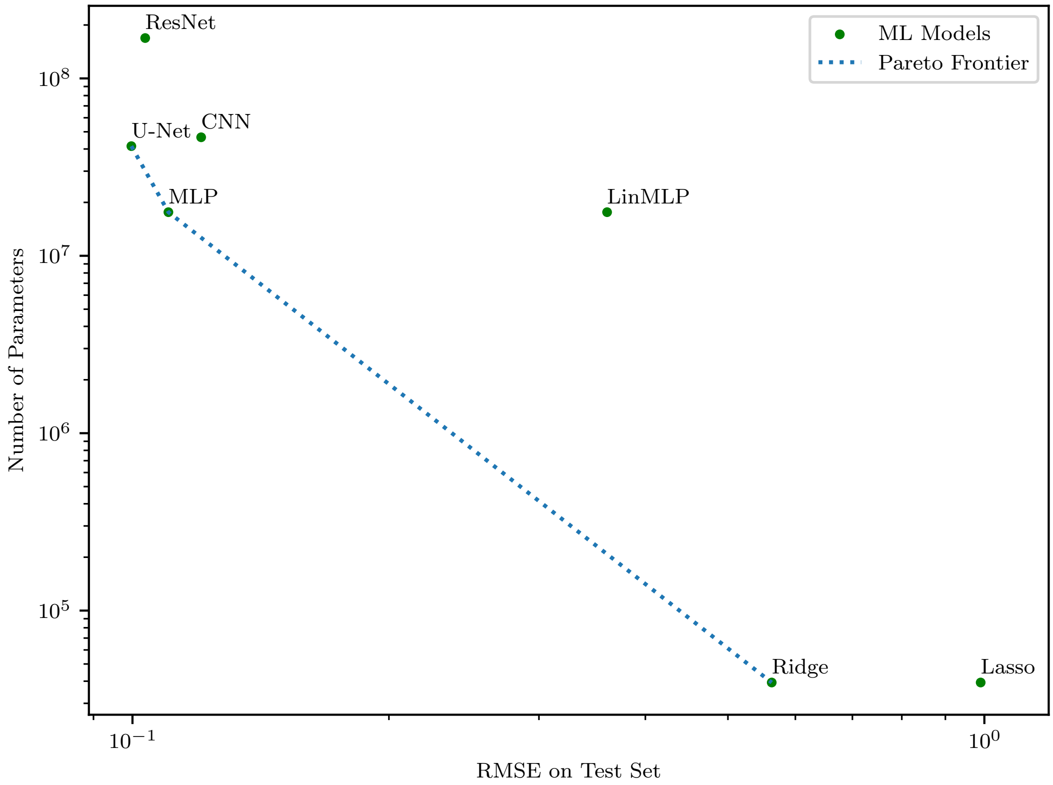


**Figure 6.** Complexity, measured by the number of parameters, is plotted against the RMSE on the test set. The Pareto frontier is visualized as the blue dotted line.

The monthly mean spatial precipitation distribution of the high-resolution reference data (NARVAL) and the simulations with the convectional cumulus scheme, the ablated U-Net, and the full U-Net are shown in Figure 7.

The data displayed in the top row and for the four rows below are not directly comparable as the initial times are different (2013/2016 for NARVAL vs. 1979 for the other plots). The position of the ITZC, for example, is strongly dependent on the season (boreal summer vs. austral summer). However, one can see that the conventional scheme tends to underestimate the mean intensity and produces too much precipitation over land and very scarce precipitation over the ocean where the high-resolution data shows most of precipitation. For the ablated U-Net we see higher precipitation values with more reasonable structures. Especially over the ocean there is a big difference to the conventional scheme, while the precipitation predictions look too spatially homogeneous, the ML-scheme predicts most of the precipitation over ocean, as does the high-resolution reference.

For month 2, a few grid cells with overly high mean precipitation are visible. This can be seen to a larger extent for the full U-Net, although in general, it predicts more than two orders of magnitude less precipitation than the ablated U-Net and the conventional scheme. The scarce places where the coupled full U-Net shows precipitation are constrained to one or a few grid cells, slightly similar to month 2 for the ablated U-Net but to a much larger extent.

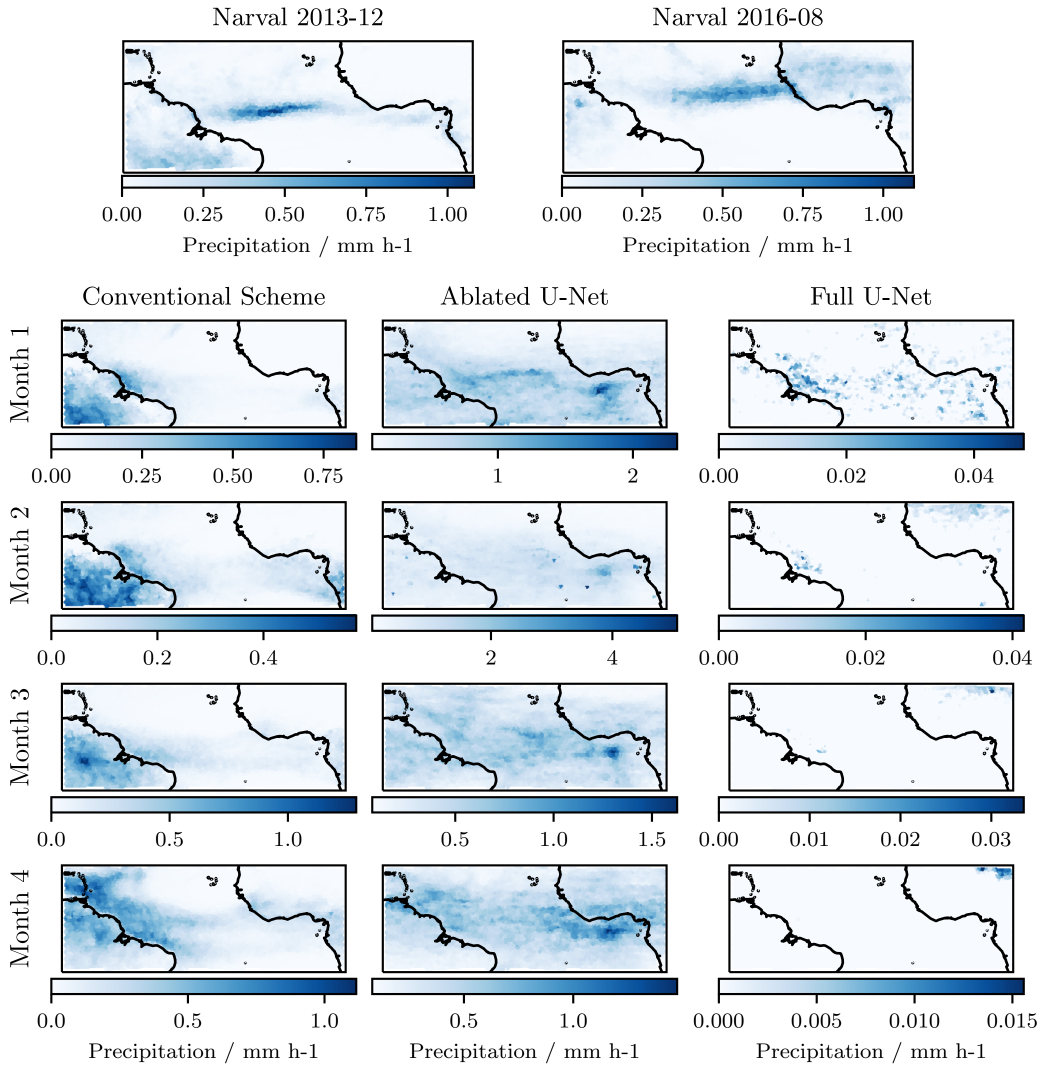


**Figure 7.** The monthly mean spatial precipitation distribution of the NARVAL data and the simulations with the convectional cumulus scheme, the ablated U-Net, and the full U-Net. For the latter three simulations the first four month of the simulations are shown. All data displayed is taken from the first ensemble member each.

## Section S2

This section will give some really short background information on the non-deep learning models used in the study. As lowest complexity models we used linear methods such as Lasso (Tibshirani, 2018) and Ridge (Hoerl & Kennard, 1970) regression. These methods are a form of linear regression with additional $L^1$ and $L^2$ regularization terms. We also compared three different models based on ensembles of decision trees: Random Forests (RF) (Breiman, 2001), Extra Trees (ET) (Geurts et al., 2006), and Gradient Boosted Trees (GBT) (Friedman, 2002). An RF is a collection of decision trees fitted on subsets of the training data and feature set. The ET model is based on the same principle but does not sub-sample the training data set, and the splitting of individual nodes in the trees is not based on the minimization of the error but it first splits at random points for random features and only afterwards chooses the best split among these candidates (Pedregosa et al., 2011). GBTs are a part of the more general family of Gradient Boosting algorithms. This family is based on ensembles of weak learners which are fitted iteratively to the residual of the previously fitted model with respect to the target data. In the case of GBTs, the class chosen as a weak learner is a decision tree. In this study we chose to use an implementation called the Histogram-based Gradient Boosting Regression Tree (Ke et al., 2017). This model is much faster for large data sets than classic GBTs because it bins the input data first, which makes the splitting step computationally much more efficient (Alsabti et al., 1998).

**Section S3**

For the Hyperparameter optimization we used the `Ray Tune` library (Liaw et al., 2018). The procedure is illustrated in Figure 8.

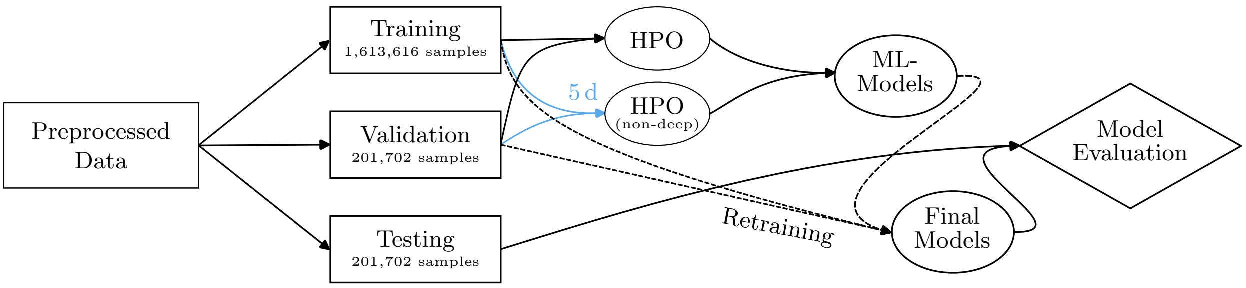


**Figure 8.** Visualization of training procedure. The preprocessed data set is split 80 %/10 %/10 % into training/validation/test data sets. The models are fit to the training data set, and validated with the validation set in the hyperparameter optimization (HPO). For the non-deep learning methods only 5 days are used for the HPO. The resulting hyperparameter-optimized models are then retrained on the full training and validation sets and evaluated mainly based on the coefficient of determination using the test data set.

**Deep Learning Models**

The number of trainable parameters for the non-ablated deep learning architectures can be seen in Table 1.

Table 2 lists the hyperparameters which are common to all deep learning models. Additionally to the listed parameter ranges in Table 2, we varied the parameter spaces described in the following for the deep learning architectures used. The parameters with the lowest error on the validation data set are marked by an asterisk.

### *MLP*

For the MLP network we vary the number of layers $n_l$, the number of neurons in each hidden layer $n_{\text{hidden}}$, and whether there is a batch normalization layer after each hidden layer with the boolean parameter $b$.

The corresponding ranges are $n_l \in \{1, 2, 3, 4, 5^*, 6\}$, $n_{\text{hidden}} \in \{16, 32, 64, 128, 256, 512, 1024, 2048^*\}$, and $b \in \{0, 1^*\}$. The optimal values for the common hyperparameters were the learning rate 0.0003, the activation leaky_relu, and the batch size 1024.

The LinMLP architecture was chosen as the best performing MLP where all activation functions are replaced by identity functions.

### *CNN*

The CNN network also has the parameters $n_l$ and $n_{\text{hidden}}$. The number of neurons per hidden layer is optimized over the same range as the MLP model, and the number of layers is varied over $n_l \in \{0, 1^*, 2, 3, 4, 5\}$. Additionally, there is a parameter for the number of channels for the convolutional layer in the beginning of the net, $n_{\text{channels}}$, and for the kernel size of the convolution $k$.

The corresponding parameter spaces are $n_{\text{channels}} \in \{1, 8, 32, 64, 256, 512, 1024^*\}$ and $k \in \{2, 3, 4^*, 5\}$. Furthermore, the optimal values for the other hyperparameters were: $\text{lr} = 0.0001$, $\sigma = \text{selu}$, $\text{bs} = 1024$, and $n_{\text{hidden}} = 2048$.

**Table 1.** Number of Trainable Parameters Used in the Various Deep Learning Models

| Network | Number of parameters / $10^6$ |
|---|---|
| MLP | 17.6 |
| U-Net | 41.5 |
| CNN | 46.6 |
| ResNet | 168.8 |

**Table 2.** Common Parameters for the Hyperparameter Optimization of the Various Deep Learning Architectures

| Parameter | Possible values |
|---|---|
| Learning rate (lr) | 0.1, 0.01, 0.001, 0.0003, 0.0001 |
| Activation function ($\sigma$) | relu, selu, gelu, sigmoid, leaky_relu |
| Batch size (bs) | 512, 1024 |

### *ResNet*

The ResNet Network is hyperparameter-optimized with respect to the number of blocks $n_b$, the number of hidden layers per block $n_l$, the number of neurons per hidden layer $n_{\text{hidden}}$, and whether there is a batch normalization layer after each hidden layer with the boolean parameter $b$.

The parameter ranges are $n_b \in \{2, 4, 8, 10^*, 14, 16\}$, $n_l \in \{1, 2, 3, 4^*\}$, $b \in \{0, 1^*\}$, and the parameter $n_{\text{hidden}}$ does have the same range as the MLP model, with the optimal value being $n_{\text{hidden}} = 2048$. The optimal values for the other hyperparameters were: $\text{lr} = 0.0001$, $\sigma = \text{relu}$, and $\text{bs} = 512$.

### *U-Net*

For the U-Net we also vary the number of blocks $n_b$, whether there is a batch norm layer after the first/second layer of each double convolution block $b_1/b_2$, and the number of channels in the first block $n_{\text{channels}}$, which is consequently doubled in each following block.

The parameter ranges are $n_b \in \{2^*, 3, 4, 5\}$, $b_1 \in \{0, 1^*\}$, $b_2 \in \{0^*, 1\}$, and $n_{\text{channels}} \in \{2^{i_m-2}, 2^{i_m-1}, 2^{i_m}\}$, where $i_m = \lfloor \log_2 (max_{\text{channels}}/2^{n_b}) \rfloor$ and $max_{\text{channels}} = 2048$. This ensures that the maximum number of channels in the lowest (having the most number of channels in the network) block of the U-Net does not have more channels than $max_{\text{channels}}$. The optimal values for the other hyperparameters were: $\text{lr} = 0.0001$, $\sigma = \text{leaky\_relu}$, and $\text{bs} = 1024$, and $n_{\text{channels}} = 512$.

### Non-Deep-Learning Models

Parameter names in this section are based on the names in the python ML-framework Scikit-learn (Pedregosa et al., 2011). Parameters with the lowest error on the validation data set are again marked by an asterisk. For Ridge and Lasso regression, we only vary the parameter $\alpha$ between $10^{-1}$ and $10^4$ with 10 evenly spaced values on a log scale. The $\alpha$ parameter gives the weighting of the regularization term in Ridge and Lasso regression, and the optimal value for both types of regression is chosen as $\alpha = 0.1$.

For the tree-based methods RF and ET we optimize over the common parameters `bootstrap` $\in \{0, 1\}$, `max_features` $\in \{\texttt{sqrt}, 1\}$, `min_samples_split` $\in \{0.5, 0.1, 0.01\}$,

and `n_estimators` $\in \{10, 100, 200\}$. The optimized RF uses no bootstrapping, the maximum number of features considered for a split is the square root of the number of features, the minimum number of samples to split a node is $0.01 \cdot$`n_samples`, and the number of estimators is chosen as 200. For the ET model we end up with the same parameters except that all features are considered for splitting a node. The GBT model parameters are varied over `learning_rate` $\in \{0.5, 0.1^*, 0.01, 0.001\}$, the maximum number of leaves for each tree `max_leaf_nodes` $\in \{40^*, 30, 20\}$, the minimum number of samples per tree `min_samples_leaf` $\in \{20, 25^*, 30\}$, and the coefficient of the $L^2$-norm term `l2_regularization` $\in \{0^*, 0.01, 0.1\}$.

As tree-based methods can quickly become very large in memory for big data sets, we set the maximum tree depth of the methods to what was found best by the HPO on the subset of 5 days. This limits the size of the trees for subsequent training on the full data set.

## References

Alsabti, K., Ranka, S., & Singh, V. (1998). CLOUDS: A decision tree classifier for large datasets. In *Proceedings of the fourth international conference on knowledge discovery and data mining* (p. 2–8). AAAI Press.

Breiman, L. (2001). Random forests. *Machine Learning*, *45*(1), 5-32. doi: 10.1023/A:1010933404324

Friedman, J. H. (2002). Stochastic gradient boosting. *Computational Statistics & Data Analysis*, *38*(4), 367-378. (Nonlinear Methods and Data Mining) doi: https://doi.org/10.1016/S0167-9473(01)00065-2

Geurts, P., Ernst, D., & Wehenkel, L. (2006). Extremely randomized trees. *Machine Learning*, *63*(1), 3-42. doi: 10.1007/s10994-006-6226-1

Hoerl, A. E., & Kennard, R. W. (1970). Ridge regression: Biased estimation for nonorthogonal problems. *Technometrics*, *12*(1), 55-67. doi: 10.1080/00401706.1970.10488634

Ke, G., Meng, Q., Finley, T., Wang, T., Chen, W., Ma, W., ... Liu, T.-Y. (2017). LightGBM: A highly efficient gradient boosting decision tree. In I. Guyon et al. (Eds.), *Advances in neural information processing systems* (Vol. 30). Curran Associates, Inc.

Liaw, R., Liang, E., Nishihara, R., Moritz, P., Gonzalez, J. E., & Stoica, I. (2018).

Tune: A research platform for distributed model selection and training. *arXiv preprint arXiv:1807.05118*.

Pedregosa, F., Varoquaux, G., Gramfort, A., Michel, V., Thirion, B., Grisel, O., ... Duchesnay, E. (2011). Scikit-learn: Machine learning in Python. *Journal of Machine Learning Research*, *12*, 2825–2830.

Tibshirani, R. (2018). Regression Shrinkage and Selection Via the Lasso. *Journal of the Royal Statistical Society: Series B (Methodological)*, *58*(1), 267-288. doi: 10.1111/j.2517-6161.1996.tb02080.x
